# Supplementary material for: Cross Validation and Maximum Likelihood estimations of hyper-parameters of Gaussian processes with model misspecification
Source: arXiv:1301.4320 source file (2013-05-31)
Supplement: Supplementary file 1 [file supplementaryMaterial.pdf]

# Supplementary material for Cross Validation and Maximum Likelihood estimations of hyper-parameters of Gaussian processes with model misspecification

François Bachoc[a,b,*]

[a] *CEA-Saclay, DEN, DM2S, STMF, LGLS, F-91191 Gif-Sur-Yvette, France*
[b] *Laboratoire de Probabilités et Modèles Aléatoires, Université Paris VII Site Chevaleret, case 7012, 75205 Paris cedex 13*

**Abstract**

In this supplementary material, a proof is given for the virtual Leave-One-Out formulas. The expression of the gradient of the Cross Validation criterion is also given, together with a proof.

In all the supplementary material, the notations are the same as in the paper.

**Proposition 0.1.** *For $1 \leq i \leq n$:*

$$c_{i,-i}^2 = \frac{1}{(\mathbf{\Gamma}_2^{-1})_{i,i}}$$

*and*

$$y_i - \hat{y}_{i,-i} = \frac{1}{(\mathbf{\Gamma}_2^{-1})_{i,i}} (\mathbf{\Gamma}_2^{-1} y)_i.$$

*Proof.* We first show that if the formulas of the proposition are true for $i = 1$ then they are true for all $i$. Let $1 \leq i \leq n$. Let $\tilde{y}$ be the vector taken from $y$ by interchanging the $i$th and the 1st components. Then $cov_2(\tilde{y}) = \mathbf{M}^{1i} \mathbf{\Gamma}_2 \mathbf{M}^{1i}$ with $(\mathbf{M}^{1i})_{k,l}$ being 1 if $k = l$ and $\{k\} \not\subset \{1, i\}$, 1 if $\{k, l\} = \{1, i\}$ and 0 elsewhere. $\mathbf{M}^{1i}$ is the matrix interchanging components 1 and $i$ of a vector. Then, using the formulas of the proposition for $\tilde{y}$ with $i = 1$:

$$var_2(y_i | y_{-i}) = var_2(\tilde{y}_1 | \tilde{y}_{-1}) = \frac{1}{((\mathbf{M}^{1i} \mathbf{\Gamma}_2 \mathbf{M}^{1i})^{-1})_{1,1}} = \frac{1}{(\mathbf{M}^{1i} \mathbf{\Gamma}_2^{-1} \mathbf{M}^{1i})_{1,1}} = \frac{1}{((\mathbf{\Gamma}_2)^{-1})_{i,i}}.$$

*Corresponding author: François Bachoc
CEA-Saclay, DEN, DM2S, STMF, LGLS, F-91191 Gif-Sur-Yvette, France
Phone: +33 (0) 1 69 08 97 91
Email: francois.bachoc@cea.fr

Furthermore:

$$
\begin{aligned}
y_i - \mathbb{E}_2(y_i|y_{-i}) &= \tilde{y}_1 - \mathbb{E}_2(\tilde{y}_1|\tilde{y}_{-1}) = \frac{1}{((\mathbf{M}^{1i}\mathbf{\Gamma}_2\mathbf{M}^{1i})^{-1})_{1,1}}((\mathbf{M}^{1i}\mathbf{\Gamma}_2\mathbf{M}^{1i})^{-1}\tilde{y})_1 \\
&= \frac{1}{((\mathbf{\Gamma}_2)^{-1})_{i,i}}(\mathbf{M}^{1i}\mathbf{\Gamma}_2^{-1}\mathbf{M}^{1i}\tilde{y})_1 = \frac{1}{((\mathbf{\Gamma}_2)^{-1})_{i,i}}(\mathbf{M}^{1i}(\mathbf{\Gamma}_2^{-1}y))_1 = \frac{1}{((\mathbf{\Gamma}_2)^{-1})_{i,i}}(\mathbf{\Gamma}_2^{-1}y)_i.
\end{aligned}
$$

Hence it is sufficient to show the formulas for the case $i = 1$, which yields the simplest expressions. Using a formula for the inverse of a partitioned matrix (Rao, 1991, p.33), we write:

$$
\begin{aligned}
\mathbf{\Gamma}_2^{-1} &= \begin{pmatrix} 1 & \gamma_{2,1}^t \\ \gamma_{2,1} & \mathbf{\Gamma}_{2,-1} \end{pmatrix}^{-1} \qquad (1) \\
&= \frac{1}{1-\gamma_{2,1}^t\left(\mathbf{\Gamma}_{2,-1}\right)^{-1}\gamma_{2,1}} \begin{pmatrix} 1 & -\gamma_{2,1}^t\left(\mathbf{\Gamma}_{2,-1}\right)^{-1} \\ -\left(\mathbf{\Gamma}_{2,-1}\right)^{-1}\gamma_{2,1} & \left(\mathbf{\Gamma}_{2,-1}\right)^{-1}\gamma_{2,1}\gamma_{2,1}^t\left(\mathbf{\Gamma}_{2,-1}\right)^{-1} + \left(\mathbf{\Gamma}_{2,-1}\right)^{-1} \end{pmatrix}.
\end{aligned}
$$

From (1), we first get

$$
(\mathbf{\Gamma}_2^{-1})_{1,1} = \frac{1}{1-\gamma_{2,1}^t\left(\mathbf{\Gamma}_{2,-1}\right)^{-1}\gamma_{2,1}},
$$

which, together with

$$
c_{1,-1}^2 = 1-\gamma_{2,1}^t\left(\mathbf{\Gamma}_{2,-1}\right)^{-1}\gamma_{2,1},
$$

proves the first one of the formulas.

Right multiplying (1) with vector $y$ and taking the first component yields

$$
(\mathbf{\Gamma}_2^{-1})_{1,1}(y_1 - \gamma_{2,1}^t\left(\mathbf{\Gamma}_{2,-1}\right)^{-1}y_{-1}) = (\mathbf{\Gamma}_2^{-1}y)_1,
$$

which, together with

$$
\hat{y}_{1,-1} = \gamma_{2,1}^t\mathbf{\Gamma}_{2,-1}y_{-1},
$$

proves the second one of the formulas.

Let us notice that we have presented here the virtual LOO formulas in the case of simple Kriging, that is to say the case when the mean of the stationary process is zero. Indeed, it is the case of interest in the present paper. Similar virtual LOO formulas have been proved in Dubrule (1983) in the more general case of universal Kriging, for which the mean at $x$ is of the form $\sum_{i=1}^p \beta_i g_i(x)$ with known functions $g_i$ and unknown coefficients $\beta_i$. It is also shown in Dubrule (1983) how to generalize these formulas to the case of $K$-fold cross validation.

□

**Proposition 0.2.** *Let $\theta_i$ be a component of $\theta$ and $\left(\frac{\partial}{\partial\theta_i}\mathbf{\Gamma}_\theta\right)$ be the derivative of $\mathbf{\Gamma}_\theta$ with respect to $\theta_i$. Then:*

$$
\frac{\partial}{\partial\theta_i}f_{ML}(\theta) = \frac{1}{n}tr\left(\mathbf{\Gamma}_\theta^{-1}\left(\frac{\partial}{\partial\theta_i}\mathbf{\Gamma}_\theta\right)\right) - \frac{1}{y^t\mathbf{\Gamma}_\theta^{-1}y}y^t\mathbf{\Gamma}_\theta^{-1}\left(\frac{\partial}{\partial\theta_i}\mathbf{\Gamma}_\theta\right)\mathbf{\Gamma}_\theta^{-1}y
$$

*and*

$$\begin{aligned} \frac{\partial}{\partial\theta_i} f_{CV}(\theta) &= 2y^t \mathbf{\Gamma}_\theta^{-1} diag(\mathbf{\Gamma}_\theta^{-1})^{-2} diag\left(\mathbf{\Gamma}_\theta^{-1}\left(\frac{\partial}{\partial\theta_i}\mathbf{\Gamma}_\theta\right)\mathbf{\Gamma}_\theta^{-1}\right) diag(\mathbf{\Gamma}_\theta^{-1})^{-1}\mathbf{\Gamma}_\theta^{-1} y \\ &- 2y^t \mathbf{\Gamma}_\theta^{-1} diag(\mathbf{\Gamma}_\theta^{-1})^{-2} \mathbf{\Gamma}_\theta^{-1}\left(\frac{\partial}{\partial\theta_i}\mathbf{\Gamma}_\theta\right)\mathbf{\Gamma}_\theta^{-1} y. \end{aligned}$$

*Proof.* The expression of $\frac{\partial}{\partial\theta_i} f_{ML}(\theta)$ is directly obtained from the matrix-derivative formulas

$$\frac{\partial}{\partial\theta_i}\log(det(\mathbf{\Gamma}_\theta)) = tr\left(\mathbf{\Gamma}_\theta^{-1}\left(\frac{\partial}{\partial\theta_i}\mathbf{\Gamma}_\theta\right)\right) \quad (2)$$

and

$$\frac{\partial}{\partial\theta_i}\mathbf{\Gamma}_\theta^{-1} = -\mathbf{\Gamma}_\theta^{-1}\left(\frac{\partial}{\partial\theta_i}\mathbf{\Gamma}_\theta\right)\mathbf{\Gamma}_\theta^{-1}. \quad (3)$$

For $f_{CV}$, we have, with $\epsilon = diag(\mathbf{\Gamma}_\theta^{-1})^{-1}\mathbf{\Gamma}_\theta^{-1} y$, and making an extensive use of (3),

$$\begin{aligned} \frac{\partial}{\partial\theta_i}\epsilon &= \left(\frac{\partial}{\partial\theta_i} diag(\mathbf{\Gamma}_\theta^{-1})^{-1}\right)\mathbf{\Gamma}_\theta^{-1} y + diag(\mathbf{\Gamma}_\theta^{-1})^{-1}\left(\frac{\partial}{\partial\theta_i}\mathbf{\Gamma}_\theta^{-1}\right) y \\ &= -diag(\mathbf{\Gamma}_\theta^{-1})^{-1}\left(\frac{\partial}{\partial\theta_i} diag(\mathbf{\Gamma}_\theta^{-1})\right) diag(\mathbf{\Gamma}_\theta^{-1})^{-1}\mathbf{\Gamma}_\theta^{-1} y - diag(\mathbf{\Gamma}_\theta^{-1})^{-1}\mathbf{\Gamma}_\theta^{-1}\left(\frac{\partial}{\partial\theta_i}\mathbf{\Gamma}_\theta\right)\mathbf{\Gamma}_\theta^{-1} y \\ &= diag(\mathbf{\Gamma}_\theta^{-1})^{-1} diag\left(\mathbf{\Gamma}_\theta^{-1}\left(\frac{\partial}{\partial\theta_i}\mathbf{\Gamma}_\theta\right)\mathbf{\Gamma}_\theta^{-1}\right) diag(\mathbf{\Gamma}_\theta^{-1})^{-1}\mathbf{\Gamma}_\theta^{-1} y \\ &- diag(\mathbf{\Gamma}_\theta^{-1})^{-1}\mathbf{\Gamma}_\theta^{-1}\left(\frac{\partial}{\partial\theta_i}\mathbf{\Gamma}_\theta\right)\mathbf{\Gamma}_\theta^{-1} y, \end{aligned}$$

which completes the proof with $\frac{\partial}{\partial\theta_i}(\epsilon^t\epsilon) = 2\epsilon^t\left(\frac{\partial}{\partial\theta_i}\epsilon\right)$.

□

## References

Dubrule, O., 1983. Cross validation of Kriging in a unique neighborhood. Mathematical Geology 15, 687–699.

Rao, C., 1991. Linear Statistical Inference and its Applications. Wiley, New York.
